# Supplementary material for: Augmented Box Replay: Overcoming Foreground Shift for Incremental Object Detection
Source: arXiv:2307.12427 source file (2023-07-23)
Supplement: Supplementary file 1 [file false_pos.tex]

\begin{figure*}[tbp]
% \vspace{-5pt}
  \centering
  % \vspace{-10pt}
  \begin{subfigure}[b]{0.32\linewidth}
    \includegraphics[width=\linewidth,height=0.6\linewidth]{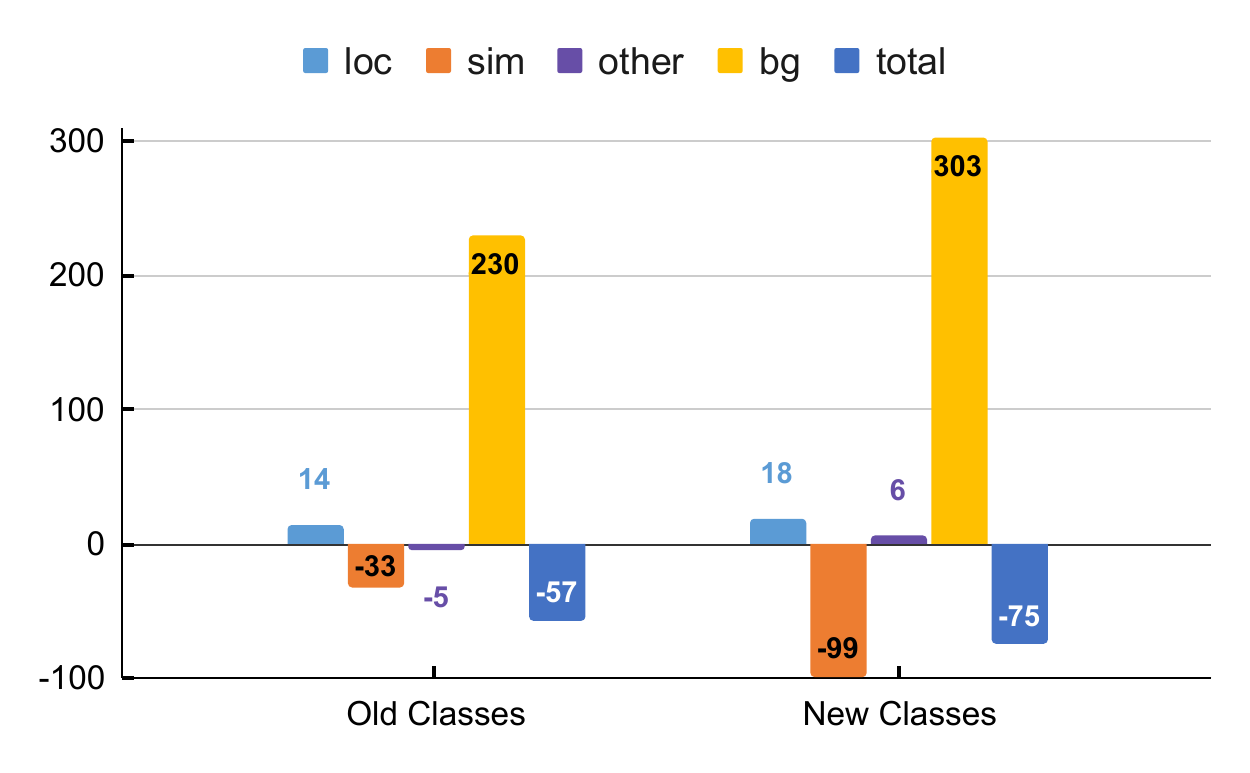}
    \caption{JT-Ours}
  \end{subfigure}
  \begin{subfigure}[b]{0.32\linewidth}
    \includegraphics[width=\linewidth,height=0.6\linewidth]{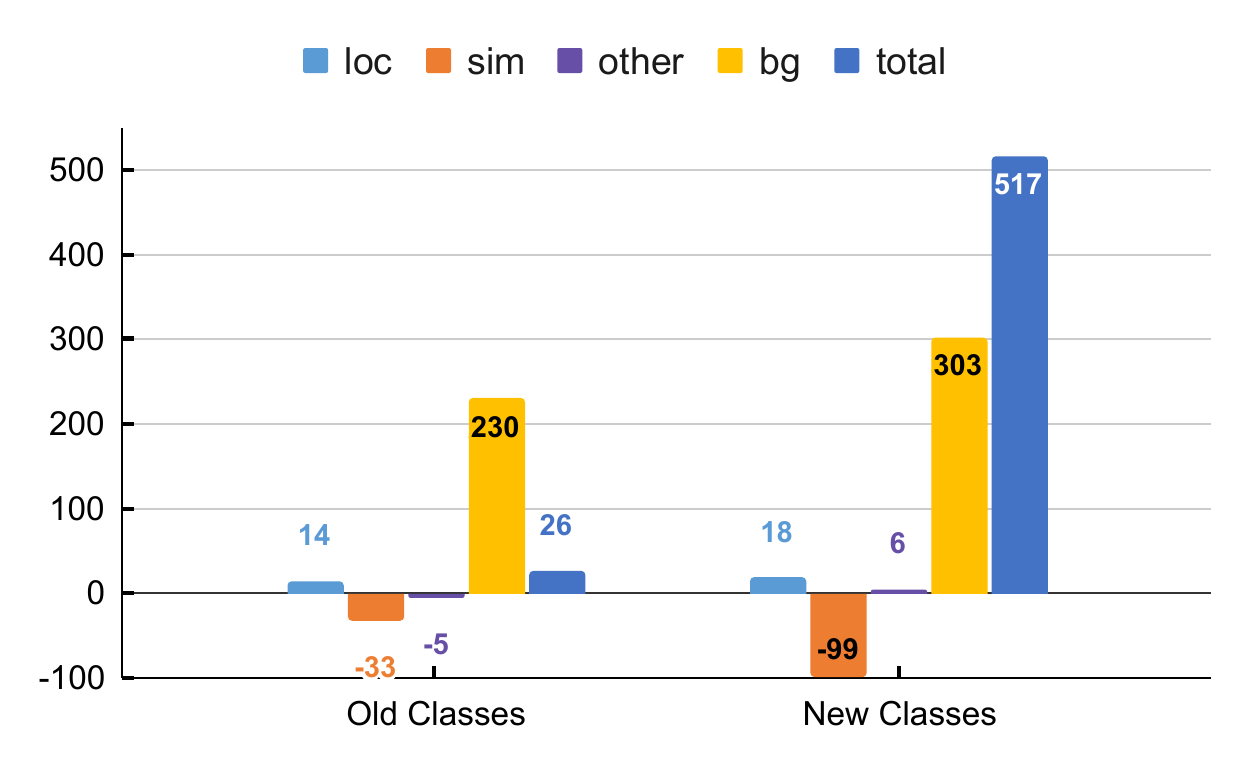}
    \caption{MMA-Ours}
  \end{subfigure}
  % \vspace{-5pt}
  \begin{subfigure}[b]{0.32\linewidth}
    \includegraphics[width=\linewidth,height=0.6\linewidth]{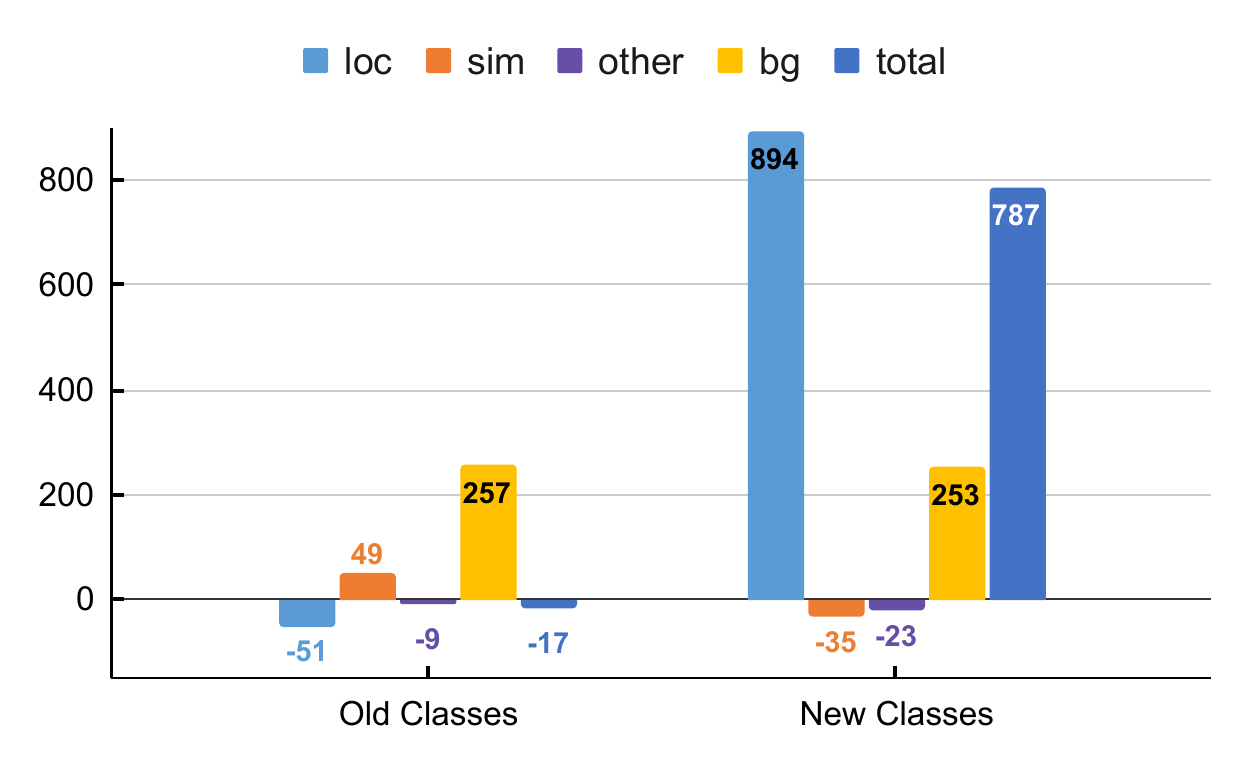}
    \caption{Image-Ours}\label{fig:imageours}
  \end{subfigure}
  % \vspace{-8pt}
  \caption{The False Positive Analysis pairwise $\uparrow$ between our proposed ABR and different algorithms in VOC 10-10 from localization error (loc), similar objects error (sim), confusion with background (bg), other type (other) and total.}
    \label{fig:fp}
\end{figure*}
