# Supplementary material for: Augmented Box Replay: Overcoming Foreground Shift for Incremental Object Detection
Source: arXiv:2307.12427 source file (2023-07-23)
Supplement: Supplementary file 2 [file imple_details.tex]

\section{Implentation details}
\subsection{Hyperparmeters}
